# Supplementary material for: A multigrid/ensemble Kalman Filter strategy for assimilation of unsteady flows
Source: arXiv:2012.10091 source file (2020-12-18)
Supplement: Supplementary file 1 [file additionalMaterialByGabriel.tex]

\section{\textcolor{cyan}{I have not touched the article from here on}}

where $F^a$ and $F^v$ represent the advective and viscous terms, respectively. A general form of the discretized representation of equation \eqref{eq:burgers_compact} can be written as:
\begin{equation}
 u_{k}=u_{k-1}+F^a_x(u_{k-1})+F^v_x(u_{k-1})\label{eq:burgers_compact_discre}
\end{equation}
The multiple numerical flux terms that affect \eqref{eq:burgers_compact} ($F^a_x$ and $F^v_x$) can be assembled in a single term $\Phi_k$ and the discretized form of the equation is represented as:
\begin{equation}
 u_{k}=u_{k-1}+\Phi_k(u_{k-1})\label{eq:burgers_compact_discre_compact}
\end{equation}
Equation \eqref{eq:burgers_compact_discre_compact} is reminiscent of the dynamical systems used in control theory (REF). It should be noted that the term $\Phi_k$ represents the discretization strategy used, as well as the model in itself. All the different fluid dynamics models analysed in this work can be written following the general 
form described in \eqref{eq:burgers_compact_discre_compact}.

To address the computational cost limitations associated with the application of the KF to compressible flows it is necessary to resort to model reduction techniques. The two major model reduction modifications that we want to implement rely on the two following hypothesis:
\begin{enumerate}
    \item The grid resolutions used in the compressible flow simulation framework are often extremely fine, which is necessary to capture the complete dynamics of the physical system. However, the type of mesh resolutions attainable through experimental measurement, such as Particle Image Velocimetry (PIV) for example, is orders of magnitude lower [REF]. In addition, the large coherent flow structures captured through direct measurement, which dictate the global dynamics of the flow [REF and some more information, maybe interesting], are sufficiently well defined with coarser resolutions. In conclusion, there are strong arguments for the application of the KF algorithm in a multiple grid framework where the state transition calculations are performed in a fine grid and the statistical modifications of the flow are performed in a secondary coarser grid. [ADD a FIGURE MAYBE]
    \item Consider a compressible flow phenomena analysed under experimental considerations. Usually, the available measurement information is limited to an observation window that represents a small region of the complete physical system. Would this experimental data be integrated into a numerical simulation, it would still represent a relatively small region when compared to the computational domain. The application of the full KF would entail a complete representation of the error covariance matrix of the whole domain. In practical applications, this is rarely achievable; even the accurate representation of the error observation matrix, limited in size to the observation window, can be problematic. It is necessary to resort to physical considerations. In some dynamical systems, the variables become spatially uncorrelated beyond some characteristic separation. Consequently, there is a strong case for the brute truncation of the error covariance matrix. That is, the domain where the KF applies, or the error space, could be reduced drastically. In practice, the error space can be created around the observation window and its size should be defined taking into account the spatial correlation of the flow. Beyond the error space, the KF no longer modifies the flow. The idea presented here is analogous to the \textit{Covariance Localization} technique which has been used in EnKF estimators [REF].
\end{enumerate}
In conclusion, the reduced-order KF methodology that we implemented can be summarized into two main aspects: the usage of multiple grids, fine and coarse, and the truncation of the error covariance matrix by reducing the actual size of the error space.

Let us define two spaces or grids that describe the same physical phenomena $x_k$ at an instant $k$. Let $x_k$ on the first space be defined as $x_k^F$, where $F$ stands for the representation of the phenomena on the fine grid. Consider that the current time-step of the phenomena has been calculated from a previous instant $k-1$ with the state-transition model. Let $x_k$ on the second space be defined as a projection of the fine grid representation on the coarse grid $x_k^C=\Pi^{F\rightarrow C}(x_k^F)$, where $\Pi$ is a projection operator. Consider now that observation $z_k^C$ at an instant $k$ is available on a coarse grid and the KF is to be applied in order to correct the representation of the phenomena on the fine space $x^F_k$. Considering the hypothesis discussed in the previous paragraph, the framework now presented allows for the application of the KF on the coarse grid, where $x_k^C$ and $z_k^C$ are integrated and a KF estimate $\hat{x}_k$ is obtained. In practice, the developed Multiple Grid KF algorithm can be conceptualized as a two-phase process:
\begin{enumerate}
  \item A predictor phase, where the state of the system at a previous time-step is used to obtain an \textit{a priori} estimate at the current instant. The estimation of $x$ is performed on the fine grid while the estimation of the error covariance is performed on the coarse grid.
  \begin{eqnarray}
    &\hat{x}_{k|k-1}^F=\Phi_k^F\hat{x}_{k-1|k-1}^F\label{eq:x_mdl_kfmg}\\
    &\hat{x}_{k|k-1}^C=\Pi^{F\rightarrow C}(\hat{x}_{k|k-1}^F)\label{eq:x_pFCmg}\\
    &P_{k|k-1}^C=\Phi_k^C P_{k-1|k-1}^C {(\Phi_k^C)}^T+Q_k^C \label{eq:Pkfmg}
  \end{eqnarray}
  \item An update step, where observation is combined with the \textit{a priori} estimate to obtain an optimal \textit{a posteriori} prediction on the coarse grid:
  \begin{eqnarray}
    &K_k^C=P_{k|k-1}^C{(H_k^C)}^T(H_k^C P_{k|k-1}^C {(H_k^C)}^T+R_k^C)^{-1}\label{eq:K_kfmg}\\
    &\hat{x}_{k|k}^F=\hat{x}_{k|k-1}^F + \underbrace{\Pi^{C\rightarrow F}\big  (K_k^C(z_k^C-H_k^C\hat{x}_{k|k-1}^C)\big)}_\text{KF Correction}\label{eq:x_kfcmg}\\
    &P_{k|k}^C=(I^C-K_k^C H_k^C)P_{k|k-1}^C\label{eq:Pc_kfmg}
  \end{eqnarray}
\end{enumerate}
Note that the superscripts $F$ and $C$ indicate if the variable which they accompany is represented on the fine or the coarse grid, respectively. It is straightforward to recognize the canon form of the KF in the Multiple Grid KF algorithm that we present. The major difference is that the KF correction is calculated not on the same space as where the state-transition is performed, but on a projection of a coarser version of this space. The coarse KF correction is then projected back on the fine space.

Equation \eqref{eq:Pkfmg} describes the \textit{a priori} estimation of the error covariance matrix. As stated before, this matrix operation scales with $N_C^3$ where $N_C$ is the dimension of the state vector $x^C_k$. Even on the reduced-order framework that we propose, \eqref{eq:Pkfmg} is problematic in terms of computational cost. Moreover, the state-transition of the covariance is performed on a coarse space $\Phi_k^C$, and the discretization errors can be significant, disrupting the covariance propagation in the system. In addition, the model error covariance $Q_k^C$ is imperfectly known, and usually estimated as proportional to a coefficient multiplied by the identity matrix $I$. Finally, the state-transition operator remains highly non-linear. The sum of the aforementioned factors can potentially render the covariance estimation unstable and the development of spurious cross-correlations is inevitable. Some authors propose [REF] a fixed error covariance matrix, so that \eqref{eq:Pkfmg} becomes:
\begin{equation}
    P_{k|k-1}^C=\Phi_k^C P_{k-1|k-1}^C {(\Phi_k^C)}^T+Q_k^C \rightarrow P_{k|k-1}^C=P_{k-1|k}^C+Q_k^C\label{eq:P_kfmg_fixed}
\end{equation}
completely removing the propagation of the covariance with the state-transition matrix. On the one side, this simplification provides huge reductions in terms of computational cost. On the other side, the spatial action range (not sure if good term) of the KF completely depends on the proper definition of the model error covariance. 

A more elegant way to deal with the limitations concerning the propagation of the error covariance matrix is the Monte-Carlo approach proposed by Evensen (REF), the Ensemble Kalman Filter EnKF. The EnKF and its variants are nowadays amongst the most popular data-driven methods applied in high-dimensional systems (ref annual review 2018 evensen) and it has been successfully applied in different domains. It has been proven that the EnKF estimator can give reliable results with just $100$ particles, which make it extremely appealing for data-driven applications.

The Multiple-Grid KF algorithm described in equations \eqref{eq:x_mdl_kfmg}-\eqref{eq:Pc_kfmg} is used as a starting point and modified to integrate an ensemble of coarse realizations. The assimilation process is split into two sub-processes. On the first sub-process, the model forecast is propagated on the fine grid on a single simulation. If observations are available, the KF update is to be performed on a coarse grid, using the statistics ($P^e$ and $R^e$) obtained in the second sub-process.
\begin{eqnarray}
    \hat{x}_{k|k-1}^F=\Phi_k^F\hat{x}_{k-1|k-1}^F\label{eq:EnKF_mg_x_fine_prop}\\
    \hat{x}_{k|k-1}^C=\Pi^{F\rightarrow C}(\hat{x}_{k|k-1}^F)\label{eq:EnKF_mg_x_fine_prop_coarseproj}\\
    K_k^C=(P^e)_{k|k-1}^C{(H_k^C)}^T\big(H_k^C (P^e)_{k|k-1}^C {(H_k^C)}^T+(R^e)_k^C\big)^{-1}\label{eq:EnKF_mg_K_coarse}\\
    \hat{x}_{k|k}^F=\hat{x}_{k|k-1}^F + \Pi^{C\rightarrow F}\big  (K_k^C(z_k^C-H_k^C\hat{x}_{k|k-1}^C)\big)\label{eq:x_kfcmg}
  \end{eqnarray}
On the second sub-process, an ensemble of $N$ coarse grid realizations are propagated forward and the EnKF is applied systematically. In this first version of the algorithm, the first sub-process does not influence at all the EnKF, thus being completely independent. However, the EnKF provides a coarse error covariance estimate for the first sub-process. Each member $n$ of the ensemble is forward with its associated state transition matrix as
\begin{equation}
(\hat{x}_n)_{k|k-1}^C=(\Phi_n)_k^C(\hat{x}_n)_{k-1|k-1}^C\label{eq:EnKF_mg_x_ensemble_prop},
\end{equation}
and the forecast error covariance is approximated as defined in equations \eqref{eq:Ensemble_Matrix},\eqref{eq:Ensemble_Mean}, \eqref{eq:Ensemble_Anomaly} and \eqref{eq:Ensemble_P}
\begin{equation}
    (P^e)^C_{k|k-1}=(X^C_{k|k-1})(X^C_{k|k-1})^T. \label{eq:EnKF_mg_ensemble_cov}
\end{equation}
An ensemble of perturbed observations is constructed as described in equations \eqref{eq:perturbed_y}, \eqref{eq:observation_matrix} and \eqref{eq:observation_matrix_anomaly}. The error covariance matrix of the measurement error is defined with the normalized anomaly ensemble of the observations
\begin{equation}
    (R^e)^C_k=(Y_o^{'})^C_k((Y_o^{'})^C_k)^T, \label{eq:EnKF_mg_observation_matrix_errorcov}
\end{equation}
and each member of the ensemble is updated according to the classical KF method
\begin{eqnarray}
K^C_k=(P^e)_{k|k-1}^C{(H_k^C)}^T\big(H_k^C (P^e)_{k|k-1}^C {(H_k^C)}^T+(R^e)_k^C\big)^{-1},\label{eq_EnKF_mg_K_ensemble}\\
(\hat{x}_n)^C_{k|k}=(\hat{x}_n)^C_{k|k-1}+K^C_k[(y_n)^C_k-H^C_k (\hat{x}_n)^C_{k|k-1}].\label{eq:ensemble_update}
\end{eqnarray}
The forecast error covariance matrix $(P^e)^C_{k|k-1}$ is transferred every instant there is an observation to the first  sub-process, where the fine grid simulation is corrected with the error statistics calculated in the ensemble sub-process. If the analysis error covariance $(P^e)^C_{k|k}$ is required, it can be obtained from the ensemble, but it is not necessary for the algorithm to perform, as the error statistics are correctly characterized in the ensemble.

\section{Reconstruction of the error covariance matrix via sparse data}
The estimate provided by the KF algorithm is subject to uncertainties. This implies that the true state of the physical phenomena $x^{true}_k$ is completely unknown and therefore, the error in $\hat{x}_{k|k}$ must be tracked in a probabilistic fashion. The associate estimate error $\hat{e}_{k|k}$ can be defined as the difference between the estimate $\hat{x}_{k|k}$ and the true state $x^{true}_k$ of the phenomena:
\begin{equation}
    \hat{e}_{k|k}=\hat{x}_{k|k}-x^{true}_k\label{eq:e_kf}
\end{equation}

There are two parameters that directly affect $\hat{e}_{k|k}$: the error statistics of the uncertainties associated with the state-transition model $w_k$ and of the measurement error $v_k$, as described in \eqref{eq:x_mdl} and \eqref{eq:z_mdl} respectively. Under the assumption that these error statistics can be described by Gaussian Probability Density Functions (PDF), $\hat{e}_{k|k}$ can be fully described by the characteristic expected value $\mathbb{E}[\cdot]$ and an error covariance model. Providing that the state-transition model is unbiased, $\mathbb{E}[\hat{e}_{k|k}]=0$ and the statistics of $\hat{e}_{k|k}$ are characterized by a positive definite, square-symmetric matrix of size $N\times N$ where $N$ is dimension of $\hat{x}_{k|k}$, which satisfies:
\begin{equation}
    P_{k|k}=\mathbb{E}[(\hat{x}_{k|k}-x^{true}_k)(\hat{x}_{k|k}-x^{true}_k)^T]=\mathbb{E}[(\hat{e}_{k|k})(\hat{e}_{k|k})^T]\label{eq:P_kf_def}
\end{equation}

$P_{k|k}$, or the error covariance matrix describes the probabilistic behavior of the error in the KF estimate $\hat{x}_{k|k}$. Assuming that both observation and model error can be described by Gaussian PDF it follows that the KF estimate $\hat{x}_{k|k}$ is a Gaussian process $\hat{x}_{k|k}\sim \mathcal{N}(x^{true}_k,P_{k|k})$ and $\hat{e}_{k|k}\sim \mathcal{N}(0,P_{k|k})$. The diagonal elements of $P_{k|k}$ represent the error variance of each element in the vector state estimate $\hat{x}_{k|k}$ and the off-diagonal terms describe the covariance of each pair of components in $\hat{x}_{k|k}$. The error covariance is of pivotal importance. It describes the error correlations in the system and is responsible for the transferring of information between the multiple components of the state vector. For example, in the framework of sequential data assimilation, an accurate and complete $P_{k|k}$ would allow the KF algorithm to correct variables that are not directly observed. The error correlations present in $P_{k|k}$ influence the calculation of the Kalman Gain, which in turn dictates how each observed component of the state vector is corrected and how they affect the correction of their zone of influence.

It is clear that using a fixed error covariance matrix, as defined in \eqref{eq:P_kfmg_fixed}, can substantially limit the potential of the KF. The estimation of the model error covariance matrix $Q_k$ remains one of the most complex aspects of data assimilation and an open challenge in the statistics and control scientific community. One of the simplest and most robust forms for $Q_k$, proposed by different authors (REF) is a diagonal form in which the model error statistics are characterized solely by the error variance of each component of the state vector. Therefore, in the absence of a state-transition model for $P_{k|k}$, the KF correction is limited to the observed variables.

Let us consider a physical phenomena $x_k$ that is analysed with numerical simulation techniques. Consider that the state transition model used is exact and the uncertainties associated with the analysis occur from the inexact specification of the initial and boundary conditions. Consider that local, unbiased but noisy observation is available and ready to be sequentially integrated in the numerical analysis through the KF. No prior information is available for the estimation of the error covariance matrix $P_{k|k}$ nor the model error covariance matrix $Q_k$ but, the measurement error variance $\sigma_z$ is known so that $R_k=\sigma_z I$. The estimation of the model covariance matrix $Q_k$ is problematic. The canon application of the KF requires that the model error follow a gaussian process $w_k\sim \mathcal{N}(0,Q_k)$. It is not true for the case described here as the numerical prediction is completely biased. Nonetheless, the KF can still be applied with a model error covariance matrix that represents as accurately as possible the bias inherent to the numerical prediction.

One possible way to overcome the bias is to take advantage of the available observation. A crude approximation of the error in the estimate would be:
\begin{equation}
    P_{k|k}=\mathbb{E}[(\hat{x}_{k|k}-z_k)(\hat{x}_{k|k
    }-z_k)^T]\label{eq:P_kf_def_z}
\end{equation}
Nonetheless the available observation is limited to a local region of the analysis domain and thereby, the direct influence of the KF is limited to this region since the error covariance matrix is considered to be fixed \eqref{eq:P_kfmg_fixed}. However, the observation can be propagated with the model dynamics by forcing it directly in a in-stream simulation on a new state vector $y_k$. The physical system represented by $y_k$ should reflect the observation in the region where it is available. The other regions of this physical system are affected by the observation through model propagation. $y_k$ could be written as:
\begin{equation}
    y_k=\Phi_k y_{k-1}+K(z_k-y_k)\label{eq:z_prop}
\end{equation}
Equation \eqref{eq:z_prop} is reminiscent of the update equation for the KF estimate \eqref{eq:x_kf} but now the gain $K$ is considered to be equal to the unity matrix $I$. The error covariance matrix can be estimated as follows:

\begin{equation}
    P_{k}=\mathbb{E}[(\hat{x}_{k|k}-y_k)(\hat{x}_{k|k}-y_k)^T]\label{eq:P_kf_def_y}
\end{equation}

The error of the system is now estimated using $y_k$ which is a crude approximation of the true state of the system $x^{true}_k$. In conclusion, $y_k$ contains the physical meausrement information in the region defined by the observation window. This information is propagated with the state transition matrix to the other regions of the numerical domain. The information represented in $y_k$ is then compared to the \textit{a priori} estimation $x_{k|k-1}$ and $P_{k|k}$ is calculated.

The error covariance estimation can be applied to the multiple grid framework. To reduce the computation cost associated to the propagation of $z_k$, the state-transition model for $y_k$ can be constructed on a coarser grid with the conditions that the global dynamics of the system can be correctly captured on this grid. For convenience, we consider that in the following equations $y_k$ and $z_k$ share the same grid resolution. However, different meshing strategies can be used. The multiple grid KF algorithm with the in-stream estimation of the error covariance matrix can be conceptualized in a two-phase process:  

\begin{enumerate}
  \item A predictor phase, where $x_{k-1|k-1}$ is advanced through the state transition model $\Phi_k$ on the fine grid and an \textit{a priori} estimation is calculated. The observation is forced and propagated on $y_k$ and the error covariance matrix is estimated:
  \begin{eqnarray}
    &\hat{x}_{k|k-1}^F=\Phi_k^F\hat{x}_{k-1|k-1}^F\label{eq:x_mdl_kfmg_PE}\\
    &\hat{x}_{k+1|k}^C=\Pi^{F\rightarrow C}(\hat{x}_{k+1|k}^F)\label{eq:x_mdl_kfmg_PE_coarse}\\
    &y_{k}^C=\Phi_k^C y_{k-1}^C+(z_k^C-H^C_ky_{k-1}^C)\label{eq:y_md_kf}\\
    &P_{k|k}^C=(\hat{x}_{k|k-1}^C-y_{k}^C)(\hat{x}_{k|k-1}^C-y_{k}^C)^T\label{eq:P_mg_E}
  \end{eqnarray}
  \item An update phase, where observation is integrated through the Kalman Filter on the coarse grid.$y_k$ maps the flow characteristics not just on the observation window but everywhere else, allowing to construct error correlations between the observation window and the other regions of the numerical domain.
  \begin{eqnarray}
    &K_k^C=P_{k|k-1}^C{(H_k^C)}^T(H_k^C P_{k|k-1}^C {(H_k^C)}^T+R_k^C)^{-1}\label{eq:K_kfmg_PE}\\
    &\hat{x}_{k|k}^F=\hat{x}_{k|k-1}^F + \underbrace{\Pi^{C\rightarrow F}\big  (K_k^C(z_k^C-H_k^C\hat{x}_{k|k-1}^C)\big)}_\text{KF Correction}\label{eq:x_kfcmg_PE}
  \end{eqnarray}
\end{enumerate}

%Drawback of using diagonal Q (localized corrections where observation is available, no cross-correlation between the variables nor spatial correlation)
%Idea, how to prove that the estimation of P makes sense. Start a test with the true value and say that the uncertainties are coming from not knowing the exact boundary conditions. Then start a simulation with forcing the observation...

\section{Results: preliminar analyses for one-dimensional test cases}
The multiple-grid KF algorithm is tested on the viscous Burgers' 1D case described in equation \eqref{eq:burgers}. We study the temporal and spatial evolution of $u(x,t)\in\mathbb{R}^N$ as dictated by the Burgers' viscous model. The discretized form of the aforementioned equation can be represented as written in equation \eqref{eq:burgers_compact_discre_compact}. The discretization of time derivatives is performed using an explicit forward Euler scheme and a second-order centered scheme is used for the spatial derivatives. The initial state of the system is set at a constant value $u(x,0)=u_0$. The inlet boundary condition is perturbed with a time dependent sinusoidal forcing: $u(0,t)=u_0+\sum_{i=1}^{n} \epsilon_i (u_0\sin(w_i t))$, where $n$ is the number of modes used to force the inflow and $\epsilon_i$ and $\omega_i$ represent their respective relative forcing intensity and oscillation frequency. The outflow boundary conditition is defined using linear extrapolation. 

Two grid systems with the same length $L_x$ are constructed. On the first grid, a very fine resolution is set in order to finely capture the dynamics of the flow. Following the notation used in the previous sections, the flow on the fine grid at an discrete instant $k$ is defined as $u^F_k$. The second grid is coarser and the representation of the flow at an instant $k$ is defined as $u^C_k$. A twin-experiment is conducted where:
\begin{enumerate}
\item Given an initial condition $u^F_0$, the flow is propagated on the fine grid with the model dynamics $\Phi_k^F$, to a state $u^F_K$ as described in equation \eqref{eq:burgers_compact_discre_compact}. The representation of $u$ from $0\leq k \leq K$ is considered to be the \textit{True} discrete state of the system (the model is assumed exact).
\item For each calculated time-step, $u^C_k$ is obtained as a projection of $u^F_k$ on the coarse grid:
\begin{equation}
u^C_k=\Pi^{F\rightarrow C}(u^F_k)\label{eq:u_fProju_c}
\end{equation}
where $\Pi$ is a projection operator. In this study it represents a centered five-point interpolation process (Lagrange Polynomial). An observation database is built by adding artificial gaussian noise to $u_k^C$:
\begin{equation}
z^C_k=u^C_k+v_k\label{eq:obser_const}
\end{equation}
where $v_k \sim \mathcal{N}(0,R)$ and R represents the error variance.
\item A new data-drive simulation on the fine grid is started with the same initial condition $u^F_0$, but the inflow is no longer perturbed $u(0,t)=u_0$. The noisy observation data $z^C$ is integrated through the multiple-grid KF. The accuracy of the filtering process is analysed by comparing the results to the \textit{True} state of the flow.
\end{enumerate} 

\subsection{Multiple-KF Twin Experiment : one perturbation mode}
A first test is performed where total number of inlet perturbation modes is set to $n=1$. The length of the domain is defined as $L_x=10\lambda$, where $\lambda$ is the wavelength of the sinusoidal inlet forcing. The forcing intensity $\epsilon$ is set to 1$\%$, in order to have a quasi-linear evolution of the inlet perturbations. The total simulation time is $K=3t_c$, where $t_c=L_x/u_0$ represents the characteristic advection time of the system. The total number of elements in the fine grid $N_F$ is set to 800 in order to have a resolution of 80 points per wavelength on the fine grid. The resolution of the coarse grid is set to 20 points per wavelength. The CFL number ($u_0 \Delta t/\Delta x$) of the \textit{True} simulation is set to 0.02. The observation database is constructed as described before. $z_k^C$ is a random gaussian variable characterized by a mean value corresponding to the true projected value on the coarse grid and a standard deviation of $\sigma=0.05u_0$, thereby $z_k^C\sim\mathcal{N}(u_k^C,\sigma^2)$. In Fig.\ref{fig:true_noise}, the \textit{True} state of the flow is represented along with the artificially created observation $z$.
\begin{figure}[!ht]
\centering
\includegraphics[width=0.8\textwidth]{true_noise.png}
\caption{\label{fig:true_noise}Snap of the \textit{True} state of the system and the noisy observation $z$ for a total \textit{True} simulation time $t_T=1.01t_c$. The grey area from $[0\leq x \leq 1]$ depicts the actual zone where observation is available.}
\end{figure} 

The data-driven simulation is started with the same numerical configuration described for the \textit{true} simulation but, without inflow forcing. In the following, we adopt the notations used in the definition of the multiple-grid KF algorithm. We assume that the observation data are not available at every instant $k$. We consider that $z^C_k$ is available every 30$\Delta t$, which amounts to roughly 120 assimilation cycles per $\lambda$. The first observation integrated to the data-driven simulation $z^C_0$ at $t_S=0$, corresponds to the \textit{True} state at an instant $t_T=1$, where time is adimensioanlized by the characteristic advection time. We assumed that the available observation is limited to an observation window defined as $[0\leq x\leq 1]$, where the length $x$ is adimensionalized with $\lambda$.

No prior knowledge is assumed about the error covariance matrix, therefore it is initialized as $P^C_{0|0}=0$. The measurement error covariance matrix $R^C_k$ is considered to be diagonal and constant in time $R^C=\sigma^2$. In this first test, the state-transition operator $\Phi^F_k$ is considered exact. Nonetheless, the inflow boundary conditions provided in this second, data-driven calculation differ from the ones of the \textit{True} simulation and the results obtained diverge considerably. The challenge in this context is to provide an accurate model error covariance matrix $Q^C_k$ that characterizes the bias due to the boundary conditions uncertainties. Different authors [REF] propose a diagonal $Q_k$ proportional to $cI$, where $I$ is the identity matrix and $c$ is a coefficient analogous to the variance of the observation $\sigma^2$. It is interesting to analyse the influence of the prescribed model error variance $c$ in the assimilation process. If $Q^C_k$ and $R^C_k$ represent diagonal, constant in time matrices and the error covariance matrix is fixed \eqref{eq:P_kfmg_fixed}, it can be proven that $P^C_{k|k}$ reaches a quasi-steady state. Due to the diagonal form of the error covariance matrices we can directly write:
\begin{equation}
K_k^C=\frac{P^C_{k|k-1}+Q^C}{P^C_{k|k-1}+Q^C+R^C}\label{eq:Kalman_Gain_diagonal}
\end{equation}
It follows that the Kalman Gain $K^C_k$ also reaches a quasi-steady state and it entirely depends on $c$ ($Q_k^C=c I$) and $\sigma$, which is fixed for this case. An analysis of the influence of $c$ is therefore presented for different values of $K^C_k$ $[0\leq K_k^C \leq 1]$, where zero represents an infinite confidence in the model prediction ($c<<\sigma^2)$ and one represents an infinite confidence in the observation ($c>>\sigma^2$). Remember that the Kalman Gain is the relative weight given to the observation or the model prediction. The synchronization of the data-driven simulation with the \textit{True} state of the system is tracked with the integrated RMSE across the entire domain for each instant k and an averaged RMSE over the total assimilation time:
\begin{eqnarray}
	&RMSE_k=\sqrt{\sum_{i=1}^{N_f}\frac{(x^{True}_{k_i}-x^F_{{k|k}_i})^2}{N_f}}\label{eq:RMSE_k}\\
	&\overline{RMSE}=\frac{1}{K}\int^K_0\sqrt{\sum_{i=1}^{N_f}\frac{(x^{True}_{k_i}-x^F_{{k|k}_i})^2}{N_f}}dt\label{eq:RMSE_avg}
\end{eqnarray}

In Fig. \ref{fig:Kanalysis} we present the RMSE of the multiple-grid KF estimator for different Kalman Gain coefficients.
\begin{figure}[!ht]
\centering
\includegraphics[width=0.8\textwidth]{Kanalysis.png}
\caption{\label{fig:Kanalysis}Performance of the estimator in terms of the Root Mean Square Error (RMSE) for an assimilation window of two characteristic advection times. A parametric study is performed to analyse the influence of the Kalman Gain. The blue color line represents the performance of the estimator when the exact error covariance matrix is provided.}
\end{figure}
The best results are obtained when the prescribed error covariance matrix is exact (it is possible to do so in this case as the true state of the system is available), and we used this case to monitor the relative  performance of the estimator. As expected, the reconstruction of the flow is complete and instantaneous if the \textit{True} error covariance matrix is provided. In the other cases, the synchronization process is gradual. Nonetheless, this is expected as the observation data is integrated very close to the inlet and the information is propagated downstream by the state-transition operator $\Phi^F_k$. We observe that for all the cases, the RMSE over the domain is gradually reduced until the information reaches the outflow boundary of the domain, a process which requires an advection time to be completed ($t_c$). Thereafter, the measured RMSE is stabilized.

To asses the overall performance of the estimator, we present in Fig. \ref{fig:Kanalysisaverage} the $\overline{RMSE}$ for the assimilation processes in function of the Kalman Gain.
\begin{figure}[!ht]
\centering
\includegraphics[width=0.8\textwidth]{Kanalysisaverage.png}
\caption{\label{fig:Kanalysisaverage}Performance of the estimator in terms of the integrated RMSE over the entire assimilation window.}
\end{figure}
It is interesting to observe that three clear operating regimes emerge:
\begin{enumerate}
\item \textbf{Optimal Regime}. There exists an optimal steady-state Kalman Gain which minimizes the RMSE and thereby, assures the synchronization of the twin-experiment. As the measurement error variance $\sigma^2$ is fixed, the estimator is completely controlled by the error model variance coefficient $c$. The results show that for this test-case, the minimum RMSE is found when the relative confidence in the model is greater than the one given to the measurements ($\sigma^2 > c$). The actual minimum point ($K^C= 0.06$ in this case) is dictated by the noise in the measurement $\sigma$ and especially, by the frequency of the available data (120 observations per $\lambda$ in this case). The minimum RMSE point should shift to the left of the curve with a higher frequency (more confidence in the model error) and to the right with a lower frequency (less confidence in the model). In terms of absolute performance, we expect the accuracy of the estimator to weaken with sparser (in time) observation. In Fig.\ref{fig:optimalK} we present a snap of the estimator $x^F_{k|k}$ for a total simulation time of $t_S =1.15$.
\begin{figure}[!ht]
\centering
\includegraphics[width=0.8\textwidth]{optimalK.png}
\caption{\label{fig:optimalK}Snap of the estimator $x_{k|k}^F$ for $K^C=0.06$ and the \textit{True} state of the system for a total simulation time of $t_S=1.15$. The red line represents the KF Correction. The grey area from $[0\leq x \leq 1]$ depicts the actual zone where observation is available.}
\end{figure}
\item \textbf{Underprediction of the model error variance $c$.} When the model error variance is underpredicted we observe a very rapid decline in the performance of the estimator. In Fig.\ref{fig:underpredK} we present a snap of the estimator for $K^C=0.005$, an extreme case of underprediction. 
\begin{figure}[!ht]
\centering
\includegraphics[width=0.8\textwidth]{underpredictedK.png}
\caption{\label{fig:underpredK}Snap of the estimator $x_{k|k}^F$ for $K^C=0.005$ and the \textit{True} state of the system for a total simulation time of $t_S=1.15$. The red line represents the KF Correction. The grey area from $[0\leq x \leq 1]$ depicts the actual zone where observation is available.}
\end{figure}
It is interesting to notice that the signal, although in perfect phase with the \textit{True} state, is underpredicted. Since the confidence in the model is too high, the relative weight given to the observation is too small to allow the complete resynchronization of the twin-flow experiment. In conclusion, if the model error covariance matrix is underpredicted, the estimation is underpredicted but smooth.
\item \textbf{Overprediction of the model error variance $c$.}  In this operating regime, the relative weight given to the measurement is too high and the performance of the estimator is diminished. However, the loss of performance is of different nature in this case and not due to underprediction.  If the relative weight of the observations in the KF process is overpredicted, the noise present in this observations may disrupt the estimate. In extreme cases it might even affect the numerical stability of the simulation if high gradients exist. In Fig. \ref{fig:overpredK} we present a snap of the estimate for $K^C=0.80$:
\begin{figure}[!ht]
\centering
\includegraphics[width=0.8\textwidth]{overpredK.png}
\caption{\label{fig:overpredK}Snap of the estimator $x_{k|k}^F$ for $K^C=0.80$ and the \textit{True} state of the system for a total simulation time of $t_S=1.15$. The red line represents the KF Correction. The grey area from $[0\leq x \leq 1]$ depicts the actual zone where observation is available.}
\end{figure}
Notice that the high-frequency components of the observation are integrated into the model and propagated downstream through the dynamical system. Therefore, the performance of the estimator is significantly affected. 
\end{enumerate}
In conclusion, we have tested the multiple-grid KF estimator on a one-dimensional test-case with promising performance results. The limitations of the methodology used are also clear. Since we assume diagonal error covariance matrices and the propagation of the error statistics is fixed, the estimator modifies the flow only on the region where observation is present. A second drawback of the algorithm is that it depends significantly on the model error covariance matrix, which is not known a priori. Nonetheless, the twin-experiment presented in this section permits to draw important conclusions. As Evensen et al state in [REF annual review geo 2018], the model is paramount. The overall confidence given to the model should be higher than the one given to the measurements. The smoothness of the final solution is also an important factor to be monitored in the estimator. In a practical case, a convergence analysis could be performed where the control parameter is the prescribed model error variance $c$. However, the overall performance of the estimator depends significantly on the frequency of the available measurements. A smooth estimate does not inherently imply an accurate result since underprediction might still be present.
